# Supplementary material for: Game Theory on the Ground: The Effect of Increased Patrols on Deterring Poachers
Source: arXiv:2006.12411 source file (2020-06-22)
Supplement: Supplementary file 1 [file appendix.tex]

\section{Appendix}

\subsection{Impact of individual features}

\begin{figure*}
  \centering
  \includegraphics[width=0.7\textwidth]{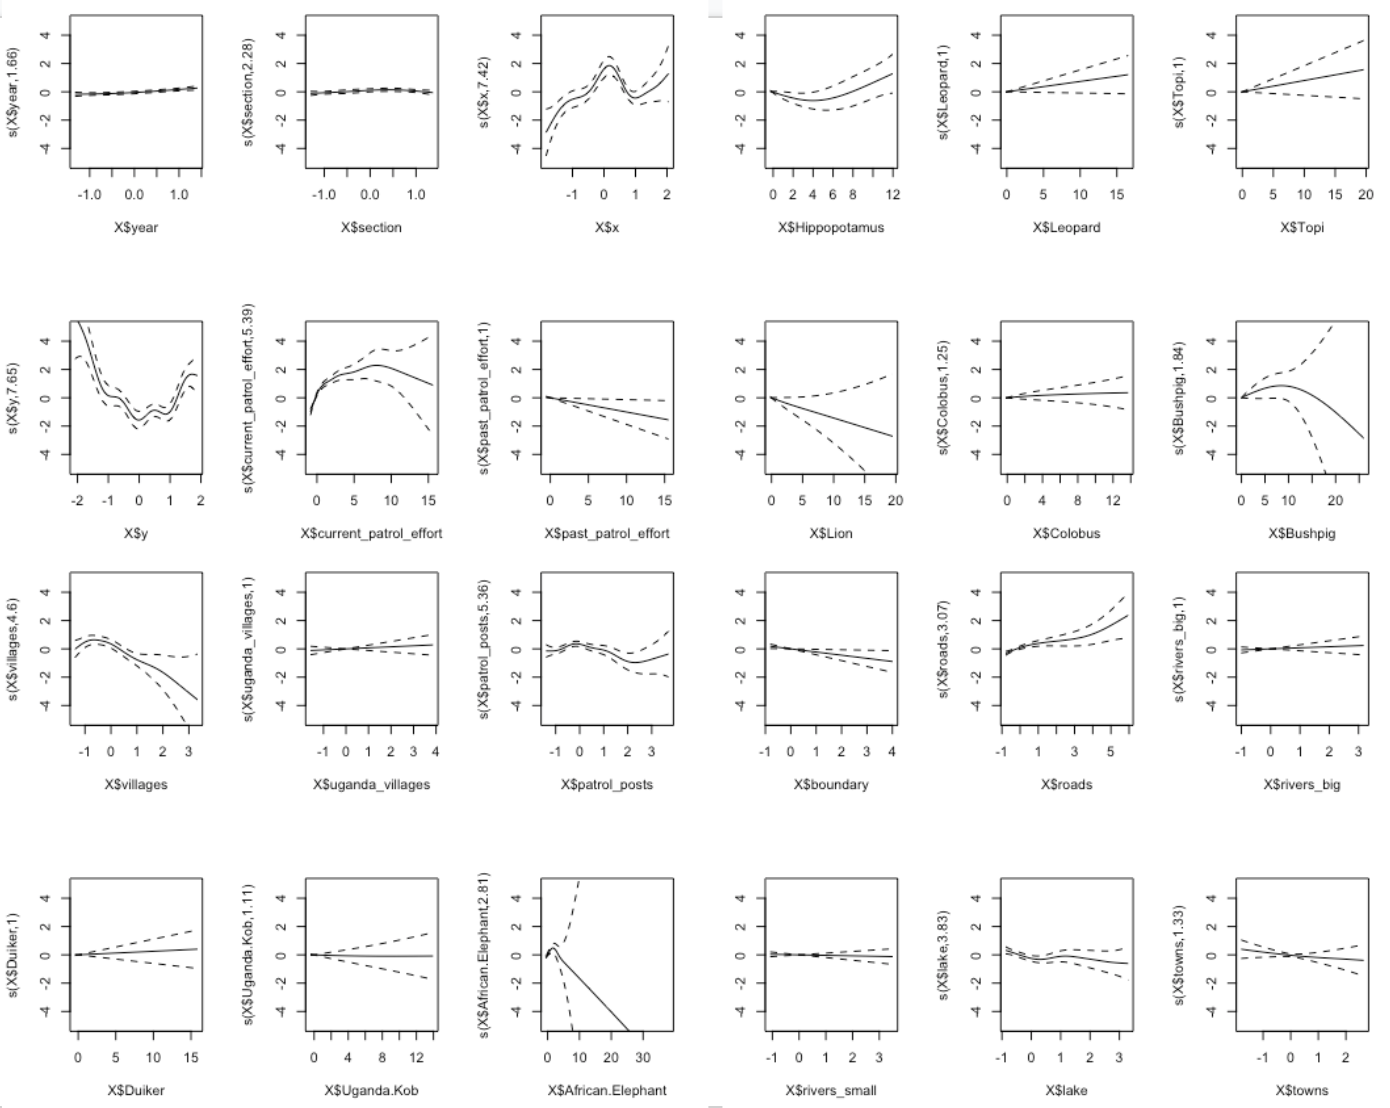}
  \caption{Component functions of each feature in the the generalized additive model. Shown are the values model estimates (solid black line) along with the 95\% confidence interval (dashed lines). {\color{red} TODO: make graphs more readable. pick which ones to show: only significant ones}}
  \label{fig:gam_components}
\end{figure*}

We learn a generalized additive model (GAM) to isolate the impact of each feature in the park on poaching activity. Unlike black-box machine learning algorithms, GAMs are interpretable in that the contribution of each independent variable is independently encoded \cite{hastie1986generalized}. Generalized linear models (GLMs) have a similar type of interpretability, but can only learn linear relationships. By contrast, GAMs learn smooth functions on each variable, which are nonparametric. 

{\color{red} need to state what you are predicting with the GAM somewhere}

For this analysis, we use the ranger observations from QENP on a timescale of 3 months. Using the \texttt{mgcv} library in R, we learn a GAM across smoothed functions of each feature. We avoid including any interaction terms, which depend on two or more variables. 

The p-value on each smooth term indicates the strength of the effect each feature has on poaching. Coming with no surprise, current patrol effort is extremely significant, with a p-value below $2 \times 10^{-16}$. Distance to roads and villages both have p-values below 0.001. Distance to patrol posts and number of African elephants are very significant, with $p < 0.01$. Additionally, past patrol effort, distance to boundary and lake, and number of hippopotamus are all significant, with $p < 0.05$. 

%{\color{red} TODO: should i include a table with the p-values of all variables? also with the $k$ and effective degrees of freedom?}

The component functions of the GAM are shown in Figure~\ref{fig:gam_components}. Consistent with the patterns observed in Section~\ref{sec:logistic-model}, the slope of past patrol effort is negative, indicating that increased ranger patrol reduces the likelihood of poaching in the next timestep. The slope of current patrol effort is also positive, which again is consistent with our expectation and earlier findings. 

To interpret the plots, note that larger absolute values indicate that feature is a strong predictor of poaching likelihood. Positive values indicate that, all else held equal, the feature is correlated with an increase in poaching probability; negative values indicate a decrease in poaching. The landscape features distance to boundary and distance to villages both have strong negative impacts on poaching, which makes sense: having to travel greater distance from the outside and from their homes would disincentivize poachers. Distance to road has a strong positive trend, which may seem counterintuitive. However, this trend can be explained by the fact that animals are unlikely to travel near roads, as wildlife tend to flee from noise. Thus, poachers will have to travel further from roads to set their snares where animals are. 

Another interesting trend can be seen in the plot of patrol posts. The function is initially slightly negative, then rises above 0, then falls back down to negative. This trend suggests that poachers avoid laying snares close to patrol posts, where rangers are based, and are more likely to poach further from these patrol posts. Further out, the decline in poaching probability might be due to the fact that areas further from patrol posts are less accessible. 

Several animals, such as leopard, topi, and Duiker are correlated with an increased likelihood of poaching.
